# Supplementary material for: Shifts: A Dataset of Real Distributional Shift Across Multiple Large-Scale Tasks
Source: arXiv:2107.07455 source file (2022-02-11)
Supplement: Supplementary file 1 [file appendix_related.tex]

\section{Comparison to Domain Adaptation or IRM Methods
}\label{apn:related}
